# Supplementary material for: PanoGRF: Generalizable Spherical Radiance Fields for Wide-baseline Panoramas
Source: arXiv:2306.01531 source file (2023-12-06)
Supplement: Supplementary file 1 [file fig_cmp_appendix_m3d.tex]

% % {"bbox": [89, 95, 830, 312]}
% \newcommand{\cropcmpmatterport}[1]{
%   \makecell{
%   % left bottom right top
%   \includegraphics[trim={89px 95px  830px 310px}, clip, width=\resultscropwidth]{#1} 
%   \\
%   \includegraphics[trim={496px 195px 399px 188px}, clip, width=\resultscropwidth]{#1} 
%   }
% }

% \cropcmpmatterport{results/cmp_m3d/ibrnet/3.png} &
% \cropcmpmatterport{results/cmp_m3d/omnisyn/3.jpg} &
% \cropcmpmatterport{results/cmp_m3d/neuray/3.jpg} &
% \cropcmpmatterport{results/cmp_m3d/panogrf/3.jpg}&
% \cropcmpmatterport{results/cmp_m3d/gt/3.jpg}  &
% \makecell[c]{
% \includegraphics[trim={0px 0px 0px 0px}, clip, width=\resultsfigwidth]{results/cmp_m3d/gt_draw/3.jpg}
% \\
% \textit{Sample 2 (Matterport3D)}
% }
